# Supplementary material for: LEGO-Motion: Learning-Enhanced Grids with Occupancy Instance Modeling for Class-Agnostic Motion Prediction
Source: arXiv:2503.07367 source file (2025-03-10)
Supplement: Supplementary file 1 [file supp.tex]

\section*{APPENDIX}

Appendixes should appear before the acknowledgment.

\section*{ACKNOWLEDGMENT}

The preferred spelling of the word ÒacknowledgmentÓ in America is without an ÒeÓ after the ÒgÓ. Avoid the stilted expression, ÒOne of us (R. B. G.) thanks . . .Ó  Instead, try ÒR. B. G. thanksÓ. Put sponsor acknowledgments in the unnumbered footnote on the first page.
